# Supplementary material for: Rapid calculation of maximum particle lifetime for diffusion in complex geometries
Source: arXiv:1801.03471 source file (2018-02-21)
Supplement: Supplementary file 1 [file Extinction_Supplementary_Revised.pdf]

# Supplementary Material: Rapid calculation of maximum particle lifetime for diffusion in complex geometries

Elliot J Carr[1] and Matthew J Simpson[1]

*School of Mathematical Sciences, Queensland University of Technology, Brisbane, Australia.*

# I. DERIVATION OF MOMENT EQUATIONS

Here we briefly outline how the system of PDEs governing the moments (Equation (2), main document), arises from the underlying random walk process. For simplicity we consider a two-dimensional Cartesian geometry, discretized with a square lattice with constant lattice spacing $\Delta > 0$. Each site is indexed in the usual way so that site $(i, j)$ has position $(x, y) = (i\Delta, j\Delta)$. Suppose a particle is placed on the lattice, and during each time step of constant duration $\tau > 0$, the particle undergoes an unbiased nearest-neighbour random walk in which the probability of the particle attempting to move during each time step is $\mathcal{P} \in [0, 1]$. Standard arguments relate this stochastic process to Equation (1) (main paper) in the limit that $\Delta \to 0$ and $\tau \to 0$ jointly, with the ratio $\Delta^2/\tau$ remaining finite. Here, $D = \mathcal{P}\Delta^2/(4\tau)$, is the diffusivity. Since we always consider a random walk where there is some absorbing boundaries present, any particle on the domain will eventually leave the system through the absorbing boundaries. Therefore, it is relevant to examine the duration of time required for all particles to leave the system. Since we deal with a stochastic model, we consider an ensemble of identically-prepared realizations, and examine the amount of time required in for the particle to leave the system in each realization.

To explore this we let $\mathbb{E}(T_{i,j})$ be the mean time for a particle released at site $(i, j)$ to exit the system. An important component of our analysis will be to consider the mean lifetime together with the higher temporal moments of the lifetime distribution. Therefore we consider $\mathbb{E}\left(T_{i,j}^k\right)$ to be the $k$th moment of the lifetime distribution of an ensemble of particles released at site $(i, j)$. The family of moments, $k = 1, 2, 3, \ldots$, can be written as

$$\mathbb{E}\left(T_{i,j}^k\right) = \sum_{l=0}^{\infty} t^k \, \mathbb{P}(T_{i,j} = t), \qquad (1)$$

where $t = l\tau$ is time, and $\mathbb{P}(T_{i,j} = t)$ is the probability that an agent released at site $(i, j)$ exits the system at time $t$. Since we know that each particle will always eventually reach the absorbing boundary, the infinite sum in Equation (1) will converge to a well-defined value.

Our aim is now to arrive at a discrete relationship for $\mathbb{E}\left(T_{i,j}^k\right)$ which can then be converted into a family of boundary value problems in the continuum limit as $\Delta \to 0$ and $\tau \to 0$ jointly,

with the ratio $\Delta^2/\tau$ remaining finite. To do this we write

$$\begin{aligned}\mathbb{P}(T_{i,j} = t) = \mathbb{P}(T_{i+1,j} = t - \tau)\frac{\mathcal{P}}{4} + \mathbb{P}(T_{i-1,j} = t - \tau)\frac{\mathcal{P}}{4} \\ + \mathbb{P}(T_{i,j+1} = t - \tau)\frac{\mathcal{P}}{4} + \mathbb{P}(T_{i,j-1} = t - \tau)\frac{\mathcal{P}}{4} \\ + \mathbb{P}(T_{i,j} = t - \tau)(1 - \mathcal{P}).\end{aligned} \tag{2}$$

The five terms on the right hand side of Equation (2) sum to give an equivalent expression by considering the five possible outcomes of the first time step of the stochastic process. These outcomes are: (i) the particle steps in the positive $x$ direction with probability $\mathcal{P}/4$; (ii) the particle steps in the negative $x$ direction with probability $\mathcal{P}/4$; (iii) the particle steps in the positive $y$ direction with probability $\mathcal{P}/4$; (iv) the particle steps in the negative $y$ direction with probability $\mathcal{P}/4$; and (v) the particle remains at the same location with probability $(1 - \mathcal{P})$. If we first consider $k = 1$, substituting Equation (2) into Equation (1), re-writing $t$ as $[(t - \tau) + \tau]$, and re-arranging, we obtain

$$\frac{\mathcal{P}}{4}\left[\mathbb{E}\left(T^1_{i+1,j}\right) + \mathbb{E}\left(T^1_{i-1,j}\right) + \mathbb{E}\left(T^1_{i,j+1}\right) + \mathbb{E}\left(T^1_{i,j-1}\right) - 4\mathbb{E}\left(T^1_{i,j}\right)\right] = -\tau, \tag{3}$$

which can be thought of as a discrete conservation statement for $\mathbb{E}\left(T^1_{i,j}\right)$. Repeating the process for $k = 2$, re-writing $t^2$ as $[(t - \tau) + \tau]^2$, leads to

$$\begin{aligned}&\frac{\mathcal{P}}{4}\left[\mathbb{E}\left(T^2_{i+1,j}\right) + \mathbb{E}\left(T^2_{i-1,j}\right) + \mathbb{E}\left(T^2_{i,j+1}\right) + \mathbb{E}\left(T^2_{i,j-1}\right) - 4\mathbb{E}\left(T^2_{i,j}\right)\right] \\ &= \binom{2}{0}(-\tau)^2 + \binom{2}{1}(-\tau)^1\mathbb{E}\left(T^1_{i,j}\right),\end{aligned} \tag{4}$$

which shows that the discrete conservation statement for the second moment is related to the first moment. Repeating the process for $k = 3$ is sufficient to observe a pattern that can be formalised by induction. In general, for $k \geq 2$, we have

$$\begin{aligned}&\frac{\mathcal{P}}{4}\left[\mathbb{E}\left(T^k_{i+1,j}\right) + \mathbb{E}\left(T^k_{i-1,j}\right) + \mathbb{E}\left(T^k_{i,j+1}\right) + \mathbb{E}\left(T^k_{i,j-1}\right) - 4\mathbb{E}\left(T^k_{i,j}\right)\right] \\ &= \sum_{l=0}^{k-1}\binom{k}{l}(-\tau)^{k-l}\mathbb{E}\left(T^l_{i,j}\right).\end{aligned} \tag{5}$$

To convert this family of discrete conservation statements into a continuum model we identify the discrete moments $\mathbb{E}\left(T^k_{i,j}\right)$ with a smooth continuous function $M_k(\mathbf{x})$. Here we will write $M_k(\mathbf{x})$ as $M_k(x, y)$. Substituting appropriate Taylor series expansions

$$\begin{aligned}M_k(x \pm \Delta, y) &= M_k(x, y) \pm \Delta\frac{\partial M_k(x, y)}{\partial x} + \left(\frac{\Delta^2}{2}\right)\frac{\partial^2 M_k(x, y)}{\partial x^2} + \mathcal{O}(\Delta^3), \\ M_k(x, y \pm \Delta) &= M_k(x, y) \pm \Delta\frac{\partial M_k(x, y)}{\partial y} + \left(\frac{\Delta^2}{2}\right)\frac{\partial^2 M_k(x, y)}{\partial y^2} + \mathcal{O}(\Delta^3),\end{aligned} \tag{6}$$

into Equation (5), and considering the limit as $\Delta \to 0$ and $\tau \to 0$ jointly with the ratio $\Delta^2/\tau$ held finite leads us to

$$D\nabla^2 M_k(\mathbf{x}) = -kM_{k-1}(\mathbf{x}), \forall k = 1, 2, 3, \ldots \tag{7}$$

where $M_0(\mathbf{x}) = 1$.

## II. ADDITIONAL RESULTS

In this section, we give additional numerical results for the test case with one obstacle. In particular, we vary our choice of the number of moments, $k$, and the specified proportion, $\varepsilon$, in the asymptotic estimate (Eq (7), Main Document), and we also vary our choice of the number of realizations in the random walk simulation (see Table I). These additional results illustrate that the asymptotic estimate (Eq (7), Main Document) exhibits rapid convergence as the numbers of moments is increased and remains accurate in the range $\varepsilon = 10^{-4}$–$10^{-1}$. Note that it is also possible to estimate the maximum particle lifetime using a random walk simulation with a smaller number of realizations, $N$, with $t^*$ taken as the $N(1-\varepsilon)$th shortest exit time. However, this method is less accurate than our asymptotic estimate (Eq (7), Main Document) and less efficient, requiring approximately 10 seconds of computation time for $N = 10,000$ on a single desktop machine, whereas solving for the first $k$ moments and applying Eq (7) (Main Document) takes less than one second across all values of $k$ and $\varepsilon$. We remark that the value of $\varepsilon$ has no effect on the computational efficiency of either approach, with the quoted runtimes in Table I equal across all values of $\varepsilon$.

| | $\varepsilon = 10^{-1} = 10\%$ | | $\varepsilon = 10^{-2} = 1\%$ | | |
|---|---|---|---|---|---|
| $k$ | $t^*$ | Particles [%] | $t^*$ | Particles [%] | Runtime [s] |
| 1 | $6.08830 \times 10^4$ | 7415 [7.415%] | $1.21766 \times 10^5$ | 443 [0.443%] | 0.054 |
| 2 | $5.50446 \times 10^4$ | 9778 [9.778%] | $1.06234 \times 10^5$ | 915 [0.915%] | 0.093 |
| 3 | $5.48132 \times 10^4$ | 9892 [9.892%] | $1.04930 \times 10^5$ | 975 [0.975%] | 0.129 |
| 4 | $5.48372 \times 10^4$ | 9885 [9.885%] | $1.04839 \times 10^5$ | 976 [0.976%] | 0.167 |
| 5 | $5.48445 \times 10^4$ | 9882 [9.882%] | $1.04835 \times 10^5$ | 976 [0.976%] | 0.203 |
| 6 | $5.48457 \times 10^4$ | 9879 [9.879%] | $1.04835 \times 10^5$ | 976 [0.976%] | 0.238 |
| 7 | $5.48458 \times 10^4$ | 9879 [9.879%] | $1.04835 \times 10^5$ | 976 [0.976%] | 0.273 |
| 8 | $5.48459 \times 10^4$ | 9879 [9.879%] | $1.04835 \times 10^5$ | 976 [0.976%] | 0.309 |
| 9 | $5.48459 \times 10^4$ | 9879 [9.879%] | $1.04835 \times 10^5$ | 976 [0.976%] | 0.347 |
| 10 | $5.48459 \times 10^4$ | 9879 [9.879%] | $1.04835 \times 10^5$ | 976 [0.976%] | 0.382 |
| RW | $5.51640 \times 10^4$ | 9719 [9.719%] | $1.06010 \times 10^5$ | 926 [0.926%] | 10.508 |
| | $\varepsilon = 10^{-3} = 0.1\%$ | | $\varepsilon = 10^{-4} = 0.01\%$ | | |
| $k$ | $t^*$ | Particles [%] | $t^*$ | Particles [%] | Runtime [s] |
| 1 | $1.82649 \times 10^5$ | 27 [0.027%] | $2.43532 \times 10^5$ | 3 [0.003%] | 0.054 |
| 2 | $1.57423 \times 10^5$ | 85 [0.085%] | $2.08612 \times 10^5$ | 6 [0.006%] | 0.093 |
| 3 | $1.55047 \times 10^5$ | 91 [0.091%] | $2.05164 \times 10^5$ | 6 [0.006%] | 0.129 |
| 4 | $1.54840 \times 10^5$ | 91 [0.091%] | $2.04842 \times 10^5$ | 6 [0.006%] | 0.167 |
| 5 | $1.54825 \times 10^5$ | 91 [0.091%] | $2.04815 \times 10^5$ | 6 [0.006%] | 0.203 |
| 6 | $1.54824 \times 10^5$ | 91 [0.091%] | $2.04812 \times 10^5$ | 6 [0.006%] | 0.238 |
| 7 | $1.54823 \times 10^5$ | 91 [0.091%] | $2.04812 \times 10^5$ | 6 [0.006%] | 0.273 |
| 8 | $1.54823 \times 10^5$ | 91 [0.091%] | $2.04812 \times 10^5$ | 6 [0.006%] | 0.309 |
| 9 | $1.54823 \times 10^5$ | 91 [0.091%] | $2.04812 \times 10^5$ | 6 [0.006%] | 0.347 |
| 10 | $1.54823 \times 10^5$ | 91 [0.091%] | $2.04812 \times 10^5$ | 6 [0.006%] | 0.382 |
| RW | $1.77348 \times 10^5$ | 32 [0.032%] | $2.22380 \times 10^5$ | 3 [0.003%] | 10.508 |

TABLE I. Estimates of the maximum particle lifetime, $t^*$, for the test case with one obstacle with $\mathcal{P} = 1$, $\delta = 0.01$, $\tau = 1$ and $\mathbf{x}_0 = (0.5, 1)$. Listed in this table are the following estimates of the maximum particle lifetime for $\varepsilon = 10^{-1}$, $10^{-2}$, $10^{-3}$, $10^{-4}$: the new asymptotic estimate (Eq (7), Main Document) for $k = 1, 2, \ldots, 10$; and an estimate of the maximum particle lifetime (denoted by RW) obtained using 10,000 random walk simulations with $t^*$ equal to the $10,000(1-\varepsilon)$th shortest exit time. The accuracy of these estimates are assessed by performing 100,000 random walk simulations and recording the number and percentage of particles that remain at $t = t^*$. The meshes used to solve Eq (2) (Main Document) are the same as those reported in the caption of Figure 1 (Main Document).
